# Supplementary material for: Heisenberg-Langevin Formalism For Open Circuit-QED Systems
Source: arXiv:1711.05699 source file (2017-11-11)
Supplement: Supplementary file 1 [file cQEDNotation.tex]

\chapter{cQED Notation}
\label{App:cQEDNotation}

In order to describe the dynamics of any cQED system we follow a common quantization procedure \cite{Bishop_Circuit_2010, Devoret_Quantum_2014}. The first step is to write the Lagrangian in terms of a generalized coordinate $\mathcal{L}[q_n]$. Then, a Legendre transformation to find the Hamiltonian in terms of the coordinate and its conjugate momentum $p_n\equiv \frac{\partial \mathcal{L}}{\partial \dot{q}_n}$ as $\mathcal{H}[q_n,p_n]=\sum\limits_n \dot{q}_n p_n -\mathcal{L}$ . Finally, we need to apply the canonical quantization by imposing a nonzero commutation relation between the conjugate pairs as  $[q_n,p_n]=i\hbar $. Here we go after the convention used in cQED by choosing the generalized coordinate as $\Phi_n(t)=\int_0^t V_n(t')\,dt'\ $ in which $V_n(t)$ is the voltage at node $n$ and is measured with respect to a ground node. This quantity has the units of magnetic flux and it can be shown that its conjugate variable has the units of charge and we denote it by $Q_n(t)$. 
There is an additional rule one has to keep in mind. In the case of external magnetic flux applied on a certain loop, the algebraic sum of flux variables over that loop should be equal to the external flux. Taking into account all these considerations, the Lagrangian for any cQED system is found as
\begin{align}
\mathcal{L}[\Phi_n ,\dot{\Phi}_n]=\mathcal{T}[\dot{\Phi}_n ]-\mathcal{U}[\Phi_n]
\end{align}
where $\mathcal{T}$ represents the kinetic energy corresponding to capacitors as $ \mathcal{T}_C[\dot{\Phi}]=\frac{1}{2}C\dot{\Phi}_C^2 $ and $\mathcal{U}$ stands for the potential energy corresponding to inductors as $ \mathcal{U}_L\{\Phi\}=\frac{1}{2L}\Phi_L^2 $ or any other nonlinear magnetic device such as Josephson junction $ \mathcal{U}_{J}[\Phi_J]=-E_J\cos\left(2\pi\frac{\Phi_J}{\phi_0}\right)$ where $\phi_0=\frac{h}{2e}$ is the flux quantum.
