# Supplementary material for: Heisenberg-Langevin Formalism For Open Circuit-QED Systems
Source: arXiv:1711.05699 source file (2017-11-11)
Supplement: Supplementary file 2 [file MultimodeJC.tex]

\chapter{Multimode Jaynes-Cummings Hamiltonian}
The classical Hamiltonian for the cQED system can be found from the circuit Lagrangian~(\ref{Eq:Full Lagrangian}) \cite{Malekakhlagh_Origin_2016}
\begin{align}
\begin{split}
\mathcal{H}_{sys}&=4\mathcal{E}_c n_j^2(t)-\mathcal{E}_j\cos{[\varphi_j(t)]}\\
&+\int_{0}^{1}dx \left\{\frac{n^2(x,t)}{2\chi(x,x_0)}+\frac{1}{2}\left[\partial_x \varphi(x,t)\right]^2\right\}\\
&+2\pi\gamma z n_j(t)\int_{0}^{1}dx\frac{n(x,t)}{\chi(x,x_0)}\delta(x-x_0),
\end{split}
\label{eqn:model-closed cQED H}
\end{align}
where $z\equiv Z/R_Q$ where $Z\equiv\sqrt{l/c}$ is the characteristic impedance of the resonator and $R_Q\equiv h/(2e)^2$ is the superconducting resistance quantum. The modification in capacitance per length originates from the system Lagrangian that contains the gauge-invariant qubit-resonator coupling $\chi_g[\dot{\varphi}_j(t)-\dot{\varphi}(x_0,t)]^2/2$. In contrast, a phenomenological product coupling $\chi_g\dot{\varphi}_j(t)\dot{\varphi}(x_0,t)$ would yield a $\mathcal{H}_{sys}$ with $\chi_s=0$ which results in bare resonator modes.

For the purpose of quantizing $\mathcal{H}_{sys}$, we find the spectrum of the resonator by solving the corresponding Helmholtz eigenvalue problem that has been discussed in Sec.~(\ref{SubApp:Spec Rep of G-closed}). We find

\begin{align}
\hat{\mathcal{H}}_{\text{sys}} \equiv \frac{\omega_j}{4}\left\{\hat{\mathcal{Y}}_j^2-\frac{\sqrt{2}}{\epsilon}\cos\left[(2\epsilon^2)^{1/4}\hat{\mathcal{X}}_j\right]\right\}+\sum\limits_{n}\left\{\frac{\omega_n}{4}\left[\hat{\mathcal{X}}_n^2+\hat{\mathcal{Y}}_n^2\right]+g_n\hat{\mathcal{Y}}_j\hat{\mathcal{Y}}_n\right\},
\label{Eq:2nd quantized closed H}
\end{align}
where have defined the canonically conjugate variables $\hat{\mathcal{X}}_l\equiv(\hat{a}_l+\hat{a}_l^{\dag})$ and $\hat{\mathcal{Y}}_l\equiv -i(\hat{a}_l-\hat{a}_l^{\dag})$, where $\hat{a}_{l}$ represent the boson annihilation operator of sector $l\equiv j,c$. Moreover, $\omega_j\equiv \sqrt{8\mathcal{E}_j\mathcal{E}_c}$ and $\epsilon\equiv\sqrt{\mathcal{E}_c/\mathcal{E}_j}$ is a measure for the strength of transmon nonlinearity. For $\epsilon=0$, we recover $\omega_j(\hat{\mathcal{X}}_j^2+\hat{\mathcal{Y}}_j^2)/4$, the Hamiltonian of a simple harmonic oscillator. In the transmon regime where $\epsilon\ll 1$, the leading contribution is $-\sqrt{2}\epsilon\omega_j\hat{\mathcal{X}}_j^4/48$. The coupling between qubit and the $n$th CC mode of the resonator is
\begin{align} 
g_n=\frac{1}{2}\gamma\sqrt{\chi_j}\sqrt{\omega_j\omega_n}\tilde{\varphi}_n(x_0).
\label{eqn:Light-Matter g_n} 
\end{align}

There are typically two approaches to diagonalize Eq.~(\ref{Eq:2nd quantized closed H}). In the first approach, assuming that the qubit nonlinearity is strong, one performs a two level reduction. Then, the multimode Rabi Hamiltonian can be derived from Eq.~(\ref{Eq:2nd quantized closed H}) by projecting the quadratures to Pauli sigma matrices, $\hat{\mathcal{X}}_j\rightarrow\hat{\sigma}^x$ and $\hat{\mathcal{Y}}_j\rightarrow\hat{\sigma}^y$, which yields
\begin{align}
\hat{\mathcal{H}}_{\text{Rabi}}=\frac{\omega_j}{2}\hat{\sigma}^z+\sum\limits_{n}\omega_n\hat{a}_n^{\dag}\hat{a}_n-\sum\limits_ng_n(\hat{a}_n-\hat{a}_n^{\dag})(\hat{\sigma}^--\hat{\sigma}^+).
\label{Eq:Rabi H}
\end{align}
In the rotating wave approximation, Eq.~(\ref{Eq:Rabi H}) transforms into the multimode Jaynes-Cummings Hamiltonian
\begin{align}
\hat{\mathcal{H}}_{\text{JC}}=\frac{\omega_j}{2}\hat{\sigma}^z+\sum\limits_{n}\omega_n\hat{a}_n^{\dag}\hat{a}_n+\sum\limits_ng_n(\hat{\sigma}^+\hat{a}_n+\hat{\sigma}^-\hat{a}_n^{\dag})
\label{Eq:JC H}
\end{align}
used in the main text. Analytic results can be found for the Purcell decay rate and the Lamb shift in the dispersive limit where $g_n\ll|\omega_j-\omega_n|$ \cite{Boissonneault_Dispersive_2009}. In a Lindblad calculation, resonator losses are included by a Bloch-Redfield approach through the Master equation for the reduced density matrix of the resonator and qubit degrees of freedom $\hat{\dot{\rho}} = -i [ \hat{\mathcal{H}}_\text{JC}, \hat{\rho} ] + \frac{\kappa_n}{2} \left( 2 \hat{a}_n \hat{\rho} \hat{a}_n^\dagger - \{ \hat{\rho}, \hat{a}_n^\dagger \hat{a}_n \} \right)$, where $\kappa_n$ can be replaced from the solutions to Eq.~(\ref{Eq:Generic NHEigfreq}). The second approach treats the nonlinearity as a weak perturbation and is explained in the next section.
